# Supplementary material for: Planning in Learned Latent Action Spaces for Generalizable Legged Locomotion
Source: arXiv:2008.11867 source file (2021-03-18)
Supplement: Supplementary file 1 [file appendix.tex]

\appendix

\section{Appendix}
\subsection{Footstep Planning Control}
\label{sec: footstep planning}

We provide some details on the footstep planner used as a baseline in our work. To calculate the desired footstep, we take the desired center of mass displacement (CoM) and orientation $(\Delta x_{com}, \Delta y_{com}, \Delta \gamma_{com})$, current location of the foot in CoM frame $(x_{f, curr}, y_{f, curr}, \gamma_{f, curr})$ and convert it to a desired footstep for each foot, assuming a tripod gait.
\begin{align*}
    \Delta x_f = \Delta x_{com} + r \cdot [\cos(\gamma_{f, curr} + \Delta \gamma_{com}) - \cos(\gamma_{f, curr}) ] \\
    \Delta y_f = \Delta y_{com} + r \cdot (\sin(\gamma_{f, curr} + \Delta \gamma_{com}) - \sin(\gamma_{f, curr}) ) \\
    r = \sqrt{x_{f,curr}^2 + y_{f,curr}^2} \\
    x_{f, des} = x_{f, curr} + \Delta x_f, \quad y_{f, des} = y_{f, curr} + \Delta y_f
\end{align*}

The desired footstep locations are passed through a footstep trajectory generator (linear trajectory in horizontal place, sinusoidal in vertical plane), and followed using inverse kinematics. This results in a desired footstep location that directly takes into account the desired orientation and displacement of the CoM. In our experiments, we find that such a representation of footstep planning can lead to a very fine control of CoM orientation and stable movement.

\subsection{Baseline Methods Implementation Detail}
\subsubsection{Model-free high-level}
For model-free high level, we use Soft Actor-Critic(SAC) as our baseline method. To reach different targets, we used goal-conditioned SAC which takes the target as part of the input, then outputs latent action. The goals for training are half of the goals for final testing.
\noindent \textbf{Velocity Tracking}: We use target velocities $[0.0,0.2]$m/s and $[0.2,0.0]$m/s as our training goals.
\noindent \textbf{Goal Reaching}: We use target goal positions $[0.0,2.0]$, $[2.0,0.0]$, $[0.0,-2.0]$ and $[-2.0,0.0]$ as our training goals.
\noindent \textbf{Trajectory Tracking}: We use first half of the trajectory for training the high level then test with full trajectory.

\subsubsection{Model-free low-level}For model-free low level, we continue to use goal-conditioned SAC to reach 4 target velocities: $[0.0,0.2]$m/s, $[0.2,0.0]$m/s, $[0.0,-0.2]$m/s, $[-0.2, 0.0]$m/s. The cost function for training the low-level policy can be formulate as: $c_4 = w_1||\mathbf{v}_{tgt} -  \mathbf{v}_{curr} || + w_2 ||\gamma_{tgt} -  \gamma_{curr} || + w_3||h_{tgt} -  h_{curr} || + w_4 ||v_{joint}||.$ The first two terms used for guiding the policy to target CoM velocity with 0 yaw; the third maintains the CoM at a certain height while the final term prevent joint shaking. Here, $[w_1, w_2, w_3, w_4] = [5.0, 1.0, 0.2, 0.001].$

\subsection{Training Hyperparameters}
\label{sec: hyperparameters}
Here we list the hyperparameters we use for baseline method comparison.
\begin{center}
 \begin{tabular}{ | c | c | c | c | c |} 
\hline
  & LAT & LIB & SAC & SAC-SAC \\
  \hline
  High-level NN size & 512*2 & & 512*2 & 512*2 \\
  \hline
  Low-level NN size & 512*2 & & 512*2 & 512*2 \\
  \hline
  Activation func & ReLU & & ReLU & ReLU \\
  \hline
  Num of samples & 10000 & 500 & 10000*3 & 10000*3 \\
  \hline
  Batch size & 512 &  & 512 & 512\\
  \hline
  Optimizer & Adam & &Adam & Adam \\
  \hline
    Learning rate & 1e-3& & 1e-3 & 1e-3 \\
    \hline
 
 \end{tabular}
\end{center}
